# Supplementary material for: Gimme That Model!: A Trusted ML Model Trading Protocol
Source: arXiv:2003.00610 source file (2020-03-03)
Supplement: Supplementary file 1 [file appendix.tex]

\definecolor{mGreen}{rgb}{0,0.6,0}
\definecolor{mGray}{rgb}{0.5,0.5,0.5}
\definecolor{mPurple}{rgb}{0.58,0,0.82}
\definecolor{backgroundColour}{rgb}{1,1,1}
\definecolor{mblack}{rgb}{0.1,0.1,0.1}
\lstdefinestyle{CStyle}{
    backgroundcolor=\color{backgroundColour},   
    commentstyle=\color{mGreen},
    keywordstyle=\color{magenta},
    numberstyle=\tiny\color{mGray},
    stringstyle=\color{mblack},
    basicstyle=\footnotesize,
    breakatwhitespace=false,         
    breaklines=true,                 
    captionpos=b,                    
    keepspaces=true,                 
    numbers=left,                    
    numbersep=5pt,                  
    showspaces=false,                
    showstringspaces=false,
    showtabs=false,                  
    tabsize=2,
    language=C
}

\begin{appendices} 
\section{Appendix}
\begin{lstlisting}[style=CStyle]
#include "examples.h"
#include <vector>
#include <fstream>
#include <iostream>
#include <numeric>
#include <algorithm>
#include <chrono>
#include <string>

using namespace std;
using namespace seal;

class Stopwatch
{
public:
    Stopwatch(string timer_name) :
        name_(timer_name),
        start_time_(chrono::high_resolution_clock::now())
    {
    }

    ~Stopwatch()
    {
        auto end_time = chrono::high_resolution_clock::now();
        auto duration = chrono::duration_cast<chrono::milliseconds>(end_time - start_time_);
        cout << name_ << ": " << duration.count() << " milliseconds" << endl;
    }

private:
    string name_;
    chrono::steady_clock::time_point start_time_;
};

void bootcamp_demo()
{	
	cout << endl << "============Company A============" << endl;
	cout << endl << "Step 1. Parameter Setting" << endl << endl;	

	EncryptionParameters parms(scheme_type::CKKS);
    size_t poly_modulus_degree = 4096;
    parms.set_poly_modulus_degree(poly_modulus_degree);
    parms.set_coeff_modulus(CoeffModulus::Create(poly_modulus_degree, { 37, 37, 35}));

    auto context = SEALContext::Create(parms);
    print_parameters(context);

	getchar();
	cout << endl << "Step 2. Send B parameters & data encoding format" << endl << endl;

	cout << " \"Input format: {age, sys, dia, cholesterol, height, weight }\"" << endl;

	getchar();
	cout << endl << "============Company B============"<< endl;
	cout << endl << "Step 3. Key Generation \n" << endl;

    KeyGenerator keygen(context);
    auto sk = keygen.secret_key();
	cout << endl << " Secret key is generated! " << endl;
	cout << endl << " Galois key is generated! " << endl;
    {
        ofstream fs("test.galk", ios::binary);
        Stopwatch sw(" GaloisKeys creation/save time");
        keygen.galois_keys_save(vector<int>{ 1, 2, 4}, fs);
    }
	
    getchar();
	cout << endl << "Step 4. Encode & Encrypt Test Data" << endl << endl;
	cout << " \"Test data : {25, 120, 80, 156, 67, 136 }, \n   \t{56, 141, 100, 428, 65, 171 }\"" << endl;

    size_t dimension = 16;
    vector<double> inputs;
    inputs.reserve(dimension);
	inputs = { 25, 120, 80, 156, 67, 136, 1, 0, 56, 141, 100, 428, 65, 171, 1, 0};
	
	vector<double> labels;
	labels.reserve(dimension/8);
	labels = {0, 1};


    // Use a scale of 2^20 to encode
    double scale = pow(2.0, 20);

    CKKSEncoder encoder(context);
    
    Plaintext pt;
    {
        Stopwatch sw("Encoding time");
        encoder.encode(inputs, scale, pt);
    }

    Encryptor encryptor(context, sk);

    // Create ciphertext 
    {
        ofstream fs("test.ct", ios::binary);

        Stopwatch sw("Encryption time");
        encryptor.encrypt_symmetric_save(pt, fs);
    }

    getchar();
	cout << endl << "Step 5. Send A Evaluation Keys & Encrypted Test Data" << endl;

	getchar();
	cout << endl << "============Company A============"<< endl;
	cout << endl << "Step 6. Compute the ML Algorithm Homomorphically on the Encrypted Test Data" << endl << endl;
    
    getchar();
    cout << endl << "Step 6-1. Encode the Model Weights" << endl << endl;

    vector<double> weights;
    weights.reserve(dimension);
	weights = { 0.072, 0.013, -0.029, 0.008, -0.053, 0.021, -5.329, 0, 0.072, 0.013, -0.029, 0.008, -0.053, 0.021, -5.329, 0 };

    Plaintext weight_pt;
    encoder.encode(weights, scale, weight_pt);

    getchar();
    cout << endl << "Step 6-2. Perform Plaintext-Ciphertext Mult." << endl << endl;

    // Load Ciphertext
    Ciphertext ct;
    {
        ifstream fs("test.ct", ios::binary);
        ct.load(context, fs);
    }

    // Create the Evaluator
    Evaluator evaluator(context);

    {
        Stopwatch sw("Multiply-plain time");
        evaluator.multiply_plain_inplace(ct, weight_pt);
    }
	   
    getchar();
    cout << endl << "Step 6-3. Perform Rotate-sum" << endl << endl;

    // Sum the slots
    {
        // Load the GaloisKeys
        ifstream fs("test.galk", ios::binary);
        GaloisKeys galk;
        galk.load(context, fs);

        Stopwatch sw("Sum-the-slots time");
        for (size_t i = 1; i <= 4; i <<= 1) {
            Ciphertext temp_ct;
            evaluator.rotate_vector(ct, i, galk, temp_ct);
            evaluator.add_inplace(ct, temp_ct);
        }
    }

    getchar();
    cout << endl << "Step 6-4. Multiply a Masking Vector to Minimize Side-information" << endl << endl;

    vector<double> mask;
    mask.reserve(dimension);
	mask = { 1, 0, 0, 0, 0, 0, 0, 0, 1, 0, 0, 0, 0, 0, 0, 0};

    Plaintext mask_pt;
    encoder.encode(mask, scale, mask_pt);
    evaluator.multiply_plain_inplace(ct, mask_pt);
    evaluator.rescale_to_next_inplace(ct);

    getchar();
    cout << endl << "Step 7. Send B the Result" << endl << endl;

    getchar();
    cout << endl << "============Company B============"<< endl;
    cout << endl << "Step 8. Decrypt the Result & Check the Quality of the Model" << endl << endl;

    Decryptor decryptor(context, sk);

    // Decrypt the result
    Plaintext pt_result;
    {
        Stopwatch sw("Decryption time");
        decryptor.decrypt(ct, pt_result);
    }

    // Decode the result
    vector<double> vec_result;
    encoder.decode(pt_result, vec_result);
    cout << "Results: " << vec_result[0] << "   &   "<< vec_result[8] <<endl;
	cout << "True Labels: " << labels[0] << "   &   " << labels[1] << endl;

    getchar();
    cout << endl << "Step 9. If the Quality seems Okay, Send Money to A." << endl << endl;

    getchar();
	cout << endl << "============Company A============"<< endl;
	cout << endl << "Step 10. Send the Model to B" << endl << endl;

	getchar();
	cout << endl << "============Company B============"<< endl;
	cout << endl << "Step 11. Compute the true result and check if A really gave a promised model" << endl << endl;

	cout << "Decrypted Result: " << vec_result[0] << "   &   "<< vec_result[8] <<endl;
    cout << "True Result: " << inner_product(inputs.cbegin(), inputs.cbegin()+8, weights.cbegin(), 0.0) << "   &   "<< inner_product(inputs.cbegin()+8, inputs.cend(), weights.cbegin()+8, 0.0)<< endl << endl;
}

int main()
{
    bootcamp_demo();
    return 0;
}
\end{lstlisting}
\end{appendices}
